# Supplementary material for: On Accelerated Methods for Saddle-Point Problems with Composite Structure
Source: arXiv:2103.09344 source file (2021-06-14)
Supplement: Supplementary file 1 [file Appendix_Framework.tex]

\section{Proof of Theorem~\ref{theorem:general_framework}}\label{Appendix_Framework}
Let us prove the Theorem~\ref{theorem:general_framework}.
\begin{proof}
% In fact, the proof of the theorem has already been presented in the main part of the article in paragraphs \hyperref[subsec_first]{"Loop 1"}-\hyperref[subsec_fourth]{"Loop 4"}.
The proof of the Theorem~\ref{theorem:general_framework} consists of three parts: firstly, we explicitly formulate that after \hyperref[subsec_first]{"Loop 1"}-\hyperref[subsec_fourth]{"Loop 4"} the algorithm get a solution to the saddle problem. Then we prove a technical statement about the polynomial dependence
 \begin{align*}
 \sigma^{(k)}\left(\varepsilon,\sigma\right) = \bf{poly}\left(\varepsilon, \sigma \right),
\tilde{\sigma}^{(k)}\left(\varepsilon,\sigma\right) = \bf{poly}\left(\varepsilon, \sigma \right), \sigma_0^{(k)}\left(\varepsilon,\sigma\right) = \bf{poly}\left(\varepsilon, \sigma \right), \tilde{\varepsilon}^{(k)}_f\left(\varepsilon\right) = \bf{poly}\left(\varepsilon\right), \delta^{(k)} \left(\varepsilon\right) = \bf{poly}\left(\varepsilon \right).
\end{align*}
 Finally, using the last statement, we show how to get the final estimates on the number of oracle calls. \\
\textbf{Solution obtained} Let us show that the random point $\hat{y}$ obtained after $\widetilde{O}\left( \left( \frac{H_1}{\mu_y} \right)^{1/2} \right)$ iterations of the \hyperref[subsec_first]{"Loop 1"} satisfies the Definition~\ref{def:saddle_solution} of $(\varepsilon, \sigma)$-solution of the saddle problem. As mentioned in the \hyperref[subsec_first]{"Loop 1"}, after $N_1$ iteration we receive an $(\varepsilon, \sigma)$-solution for function $h(y) + \max_{x \in \R^{d_x}}{-G(x,y)-f(x)}$, i.e. inequality
\begin{align*}
    h(\hat{y}) + \max_{x \in \R^{d_x}}\{-G(x,\hat{y})-f(x)\} - \min_{y\in \R^{d_y}}\max_{x \in \R^{d_x}}\{h(y) -G(x,y)-f(x)\} \leq \varepsilon
\end{align*}
holds True with probability $1-\sigma$. Which in turn is the Definition~\ref{def:saddle_solution} of an $(\varepsilon, \sigma)$-solution for saddle problems.\\
\textbf{Polynomial dependence}
Before obtaining the final estimates, it is important to prove that for all $i = 1, 2, 3$ dependences 
\begin{align}\label{proof_polynomial_dependence}
\sigma^{(i)}\left(\varepsilon,\sigma\right) = \bf{poly}\left(\varepsilon, \sigma \right),
\tilde{\sigma}^{(i)}\left(\varepsilon,\sigma\right) = \bf{poly}\left(\varepsilon, \sigma \right), \sigma_0^{(i)}\left(\varepsilon,\sigma\right) = \bf{poly}\left(\varepsilon, \sigma \right), \tilde{\varepsilon}^{(i)}_f\left(\varepsilon\right) = \bf{poly}\left(\varepsilon\right), \delta^{(i)} \left(\varepsilon\right) = \bf{poly}\left(\varepsilon \right)   
\end{align}
 are polynomial. This can be proved by induction: base holds true for $i = 1$. Then let us suppose that for $k \in \{1, 2\}$ we have
 \begin{align*}
 \sigma^{(k)}\left(\varepsilon,\sigma\right) = \bf{poly}\left(\varepsilon, \sigma \right),
\tilde{\sigma}^{(k)}\left(\varepsilon,\sigma\right) = \bf{poly}\left(\varepsilon, \sigma \right), \sigma_0^{(k)}\left(\varepsilon,\sigma\right) = \bf{poly}\left(\varepsilon, \sigma \right), \tilde{\varepsilon}^{(k)}_f\left(\varepsilon\right) = \bf{poly}\left(\varepsilon\right), \delta^{(k)} \left(\varepsilon\right) = \bf{poly}\left(\varepsilon \right).
\end{align*}
 According to paragraphs \hyperref[subsec_first]{"Loop 1"}-\hyperref[subsec_fourth]{"Loop 4"}  $\sigma^{(k+1)},\tilde{\sigma}^{(k+1)}, \sigma_0^{(k+1)}, \tilde{\varepsilon}^{(k+1)}_f, \delta^{(k+1)}$ are chosen such that \eqref{varepsilon_poly_CATD_with_prob}, \eqref{sigma_poly_CATD_with_prob} and $\sigma^{(k+1)} = \tilde{\sigma}^{(k)}$ hold true. These equations guarantee a polynomial dependence
  \begin{align*}
 \sigma^{(k+1)}\left(\varepsilon,\sigma\right) = \bf{poly}\left(\varepsilon, \sigma \right),
\tilde{\sigma}^{(k+1)}\left(\varepsilon,\sigma\right) = \bf{poly}\left(\varepsilon, \sigma \right), \sigma_0^{(k+1)}\left(\varepsilon,\sigma\right) = \bf{poly}\left(\varepsilon, \sigma \right), \tilde{\varepsilon}^{(k+1)}_f\left(\varepsilon\right) = \bf{poly}\left(\varepsilon\right), \delta^{(k+1)} \left(\varepsilon\right) = \bf{poly}\left(\varepsilon \right).
\end{align*}
 Which finishes the proof of polynomial dependence. According Paragraph~\ref{saddle_sigma_log} and last statement \eqref{proof_polynomial_dependence}, we can use notation $\widetilde{O}(\cdot)$ at all levels \hyperref[subsec_first]{"Loop 1"}-\hyperref[subsec_fourth]{"Loop 4"}, implying that the logarithmic part depends on the initial  $\varepsilon, \sigma$.\\
\textbf{Final estimates}
The only thing left to finish proof of the Theorem~\ref{theorem:general_framework} is an accurately count the number of oracle calls at each loop \hyperref[subsec_first]{"Loop 1"}-\hyperref[subsec_fourth]{"Loop 4"} of the general scheme. At each step we must take into account only three places in which the oracle can be called:
\begin{itemize}
    \item calculation of inexact oracles of functions $\vp, \psi$,
    \item searching the solution to the auxiliary problem \eqref{prox_step_inexact},
    \item step along the gradient \eqref{alg:gradient_step} of the functions $\vp, \psi$ in the Algorithms~\ref{alg:highorder_inexact},\ref{alg:restarts_inexact_notconvex};
\end{itemize}

The technique for counting the number of oracle calls is the same for $\nabla f, \nabla h, \nabla_x G, \nabla_y G$. Below we give only an example of calculation the number of oracle calls of $\nabla h$.

According to the Table~\ref{tabl:saddleproblem_steps} and paragraphs \hyperref[subsec_first]{"Loop 1"}-\hyperref[subsec_fourth]{"Loop 4"} we have
\begin{itemize}[label=\ding{212}]
    \item $\nabla h$ is called at each of $\widetilde{O}(\sqrt{H_1/\mu_y})$ iteration of \hyperref[subsec_first]{"Loop 1"} when:
    \begin{itemize}[label=\ding{212}]
        \item Algorithm~\ref{alg:restarts_inexact_notconvex} do the step along the gradient \eqref{alg:gradient_step}, it costs $\widetilde{O}(\tau_h)$ calls,
        \item auxiliary problem \eqref{eq:sub1} is solved; $\nabla h$ is called at each of $\widetilde{O}(\sqrt{H_2/\mu_x})$ iteration of \hyperref[subsec_second]{"Loop 2"} when:
        \begin{itemize}[label=\ding{212}]
            \item an inexact model of $\psi$ \eqref{eq:framework_aux_step2} is determined, it costs $\widetilde{O}(\mathcal{N}_h\left( \tau_h, H_1\right))$ calls,
            \item auxiliary problem \eqref{eq:sub2} is solved: $\nabla h$ is called at each of $\widetilde{O}(\sqrt{H_3/H_2})$ iteration of \hyperref[subsec_third]{"Loop 3"} when an inexact model of $\vp$ \eqref{eq:framework_aux_step3} is determined, it costs $\widetilde{O}(\mathcal{N}_h\left( \tau_h, H_1\right))$ calls;
        \end{itemize}
    \end{itemize}
\end{itemize}

Thus, we obtain that the estimate for the number of oracle calls $\nabla h$ has an nested structure of the form
\begin{align*}
    \nabla h \text{ - oracle calls}: \widetilde{O} \left( \sqrt{\frac{H_1}{\mu_y}} \left( \tau_h +   \sqrt{\frac{H_2}{\mu_x}}\left(\mathcal{N}_h\left( \tau_h, H_1\right) + \sqrt{\frac{H_3}{H_2}} \cdot \mathcal{N}_h\left( \tau_h, H_1\right)\right)\right)
    \right).
\end{align*}

The remaining estimates are obtained similarly. Finally, for obtaining an $(\varepsilon,\sigma)$-solution of  problem \eqref{eq:main30} it is sufficient to do the next number of oracle calls
\begin{align*}
    &\nabla f \text{ - oracle calls}: \widetilde{O} \left( \sqrt{\frac{H_1}{\mu_y}} \left( \mathcal{N}_f\left( \tau_f\right) + \sqrt{\frac{H_2}{\mu_x}}\cdot \tau_f\right)
    \right),\\
    &\nabla h \text{ - oracle calls}: \widetilde{O} \left( \sqrt{\frac{H_1}{\mu_y}} \left( \tau_h +   \sqrt{\frac{H_2}{\mu_x}}\left(\mathcal{N}_h\left( \tau_h, H_1\right) + \sqrt{\frac{H_3}{H_2}} \cdot \mathcal{N}_h\left( \tau_h, H_1\right)\right)\right)
    \right),\\
    &\nabla_x G \text{ - oracle calls}: \widetilde{O} \left( \sqrt{\frac{H_1}{\mu_y}} \left( \mathcal{N}_G^x\left( \tau_G\right) + \sqrt{\frac{H_2}{\mu_x}} \left( \tau_G + \sqrt{\frac{H_3}{H_2}}\cdot \tau_G \right)\right)
    \right),\\ 
    &\nabla_y G \text{ - oracle calls}: \widetilde{O} \left( \sqrt{\frac{H_1}{\mu_y}} \left( \tau_G + \sqrt{\frac{H_2}{\mu_x}} \left( \mathcal{N}_G^y\left( \tau_G, H_1\right) +  \sqrt{\frac{H_3}{H_2}}\cdot \mathcal{N}_G^y\left( \tau_G, H_1\right) \right)\right)
    \right).
\end{align*}
 Final estimates can be obtained by choosing the constants $H_1, H_2, H_3$ in the following way
$$H_1 = 2L_G, H_2 = 2L_f, H_3 = 2\left(L_G + \frac{L_G^2}{\mu_y + H_1}\right).
$$
\qed 
\end{proof}
